# Supplementary material for: Absence of proton tunneling during the hydrogen bond symmetrization in $\delta$-AlOOH
Source: arXiv:2110.06757 ancillary file (2021-10-13)
Supplement: Supplementary file 1 [file dAlOOH_SM.pdf]

# Supplementary Material: Absence of proton tunnelling during the hydrogen bond symmetrization in $\delta$-AlOOH

Florian Trybel,[1,2,*] Thomas Meier,[1,3] Biao Wang,[1,4] and Gerd Steinle-Neumann[1]

[1]*Bayerisches Geoinstitut, Universität Bayreuth, D-95440 Bayreuth, Germany*
[2]*Department of Physics, Chemistry and Biology (IFM), Linköping University, SE-581 83, Linköping, Sweden*
[3]*Center for High Pressure Science and Technology Advanced Research (HPSTAR), Beijing 100094, China*
[4]*Department of Earth Sciences, University of Oxford, OX1 3AN Oxford, United Kingdom*

(Dated: June 28, 2021)

* florian.trybel@liu.se

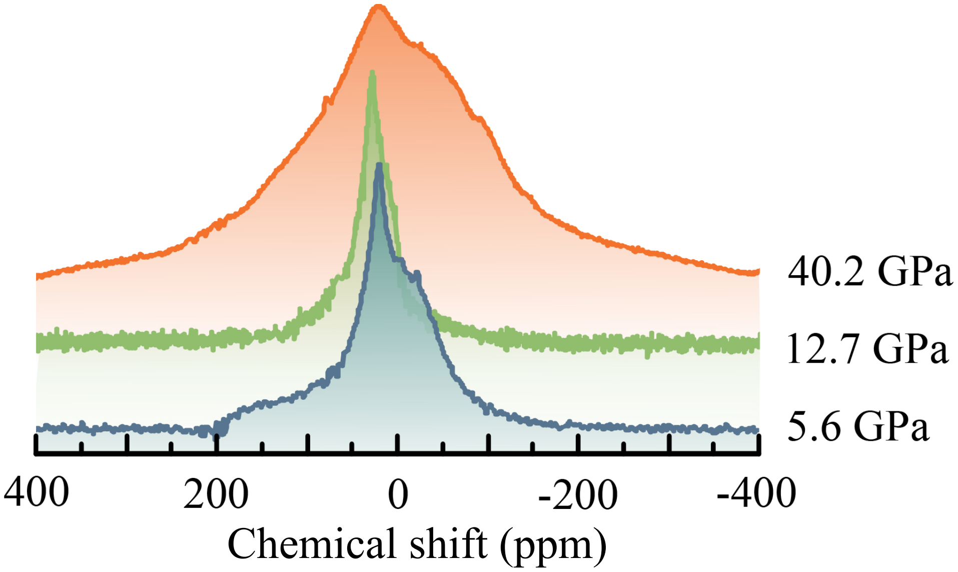


FIG. S1. Representative $^{1}$H-NMR solid-echos at 5.6, 12.7 and 40.2 GPa.

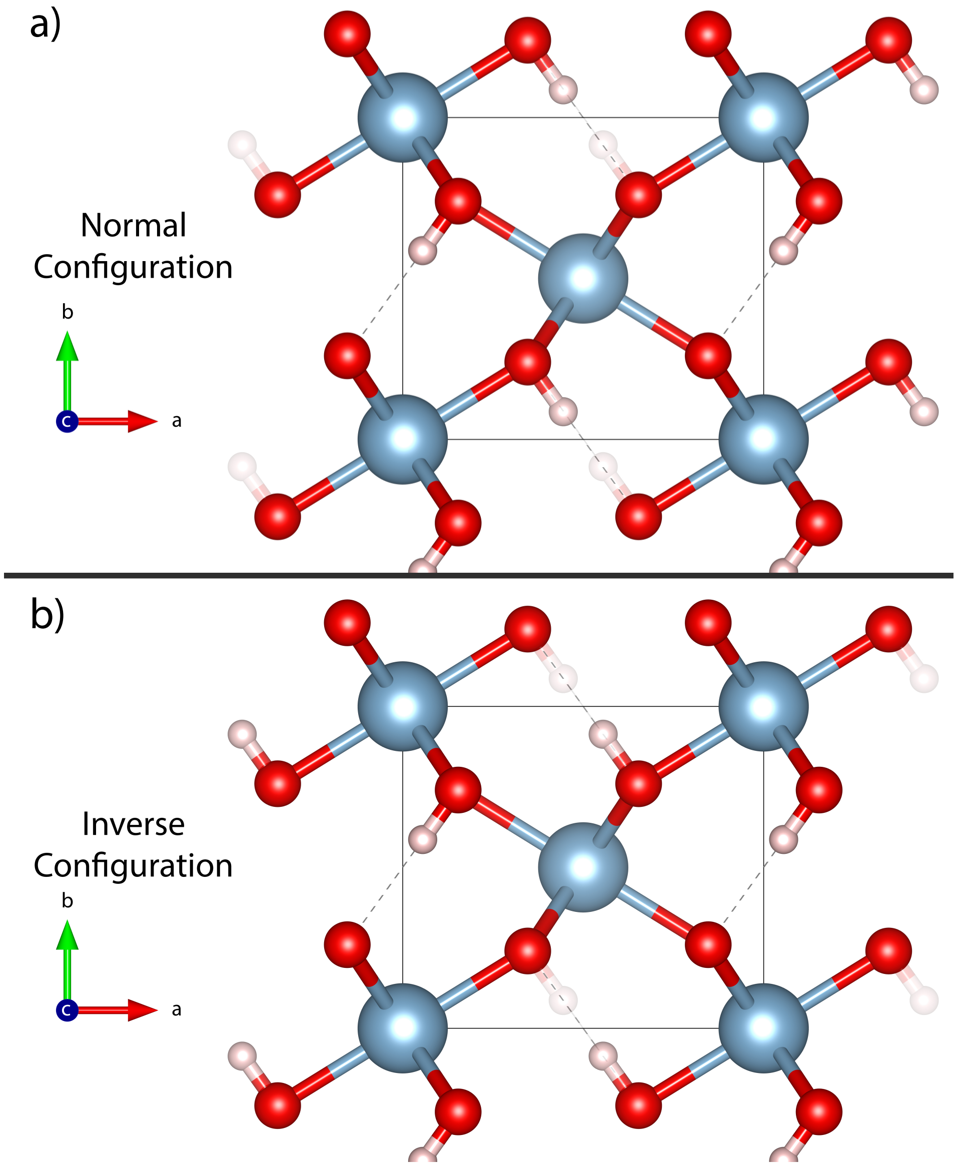


FIG. S2. Visualization of the two hydrogen position configurations used for potential sampling: **(a)** normal and **(b)** inverse sampling. Aluminum is shown in blue, oxygen in red and hydrogen in white. The hydrogen atoms with the lower opacity show the respective other configuration for easier comparison.
